# Supplementary material for: A Generalized Projected Bellman Error for Off-policy Value Estimation in Reinforcement Learning
Source: arXiv:2104.13844 source file (2024-07-31)
Supplement: Supplementary file 1 [file old_appendix.tex]

\section{A Survey of Off-Policy Algorithms for the Linear $\mspbe$}
\label{sct:Algorithms}

In this section, we describe the methods used in the empirical study that follows next. In particular, we discuss the optimization objective, and provide detailed update equations highlighting how prior or posterior corrections are used in each method. We begin with the Gradient-TD family of methods that minimize the excursion variant of the linear $\mspbe$. We then discuss modifications on GTD($\lambda$)---namely the Hybrid methods and the Saddlepoint methods. Then we discuss the second family of off-policy methods, the Emphatic methods. We conclude with a discussion of several methods that reduce variance of posterior corrections, using action-dependent bootstrapping.



\subsection[GTD and GTD2]{Gradient Temporal Difference Learning}

Gradient-TD methods were the first to achieve stability with function approximation using gradient descent \citep{sutton2009fast}. This breakthrough was achieved by creating an objective function, the linear $\mspbe$, and a strategy to sample the gradient of the linear $\mspbe$.
% whose gradient yields an update with bootstrapping. The the gradient of the linear $\mspbe$ can be rearranged to achieve this goal.
The negative of the gradient of the linear $\mspbe$, with weighting $d = d_b$, can be written:

\begin{align}\label{eq:GradientOfMSPBE}
\nabla \text{linear $\mspbe$}(\vecw) &= \mathbb{E}_{d_b}\bigl[\delta(S,A,S') \vecz(S)\bigr] \\
&- \mathbb{E}_{d_b}\bigl[\gamma(S')\vecx(S') \vecx(S)^{\tr}\bigr]  \mathbb{E}_{d_b}\bigl[\vecx(S) \vecx(S)^{\tr}\bigr]^{-1}  \mathbb{E}_{d_b}\bigl[\delta(S,A,S') \vecz(S)\bigr] \nonumber
.
\end{align}
%
Sampling this gradient is not straightforward due to the product of expectations. To resolve this issue, a second weight vector, $\vech$, can be used to estimate $\mathbb{E}_{d_b}[ \vecx_t\vecx_t^\top]^{-1}\mathbb{E}_{d_b}[\delta_t\vecz_t]$ and avoid the need for two independent samples. The resultant method, called GTD($\lambda$), can be thought of as approximate stochastic gradient descent on the linear $\mspbe$ and is specified by the following updated equations:
%
\begin{align}\label{eq:GTD}
\vech_{t+1} \leftarrow& ~\vech_t + \alpha_h\bigl[\delta_t\vecz^\rho_t - (\vech_t^{\tr}\vecx)\vecx_{t+1}  \bigr] \nonumber\\\
\vecw_{t+1} \leftarrow& ~\vecw_t + \alpha \delta_t \vecz^\rho_t - \underbrace{\alpha \gamma_{t+1} (1-\lambda)(\vech_t^{\tr}\vecz^\rho_t)\vecx_{t+1}}_{\text{correction term}}
\end{align}
%
The GTD($\lambda$) algorithm has several important details that merit further discussion.
The most notable characteristic is the second weight vector $\vech\in\mathbb{R}^k$ that forms a quasi-stationary estimate of the last two terms in the gradient of the linear $\mspbe$.
The corresponding two-timescale analysis highlights that the learning rate parameter $\alpha_h\in\mathbb{R}$ should be larger than $\alpha$, where the weights $\vecw$ change slower to enable $\vech$ to obtain such a quasi-stationary estimate \citep{sutton2009fast}. In practice, the best values of $\alpha$ and $\alpha_h$ are problem dependent, and the practitioner must tune them independently to achieve good performance \citep{white2015developing, white2016investigating}. Another important detail is that the first part of the update to $\vecw$ corresponds to Off-policy TD($\lambda$). When $\lambda = 1$, the second term---the correction term---is removed, making GTD(1) = TD(1). Otherwise, for smaller $\lambda$, the correction term plays a bigger role.


The GTD($\lambda$) algorithm has been shown to be stable with linear function approximation. The GTD($\lambda$) with $\lambda=0$, also known as TDC, has been shown to converge in expectation with i.i.d sampling of states \citep{sutton2009fast}. The convergence of Gradient-TD methods with $\lambda>0$ was later shown in the Markov noise case with constant stepsize and stepsizes that approach zero in the limit \citep{yu2017generalized}.

The GTD2($\lambda$) algorithm is related to GTD($\lambda$), and can be derived starting from the gradient of the excursion linear $\mspbe$ in Equation \ref{eq:GradientOfMSPBE}. The gradient of the linear $\mspbe$ given in Equation \ref{eq:GradientOfMSPBE} is an algebraic rearrangement of:
\begin{equation*}
\nabla \text{linear $\mspbe$}(\vecw) ~=~\mathbb{E}_{d_b} \bigl[(\vecx(S) - \gamma(S') \vecx(S'))\vecz(S)^{\tr}\bigr]  \mathbb{E}_{d_b}\bigl[\vecx(S) \vecx(S)^{\tr}\bigr]^{-1}  \mathbb{E}_{d_b}\bigl[\delta(S,A,S') \vecz(S)\bigr]
.
\end{equation*}
As before, the last two terms can again be replaced by a secondary weight vector $\vech \in \mathbb{R}^k$. The resultant expression
\begin{equation*}
\mathbb{E}_{d_b} \bigl[(\vecx(S) - \gamma(S') \vecx(S'))\vecz(S)^{\tr}\bigr]  \vech
,
\end{equation*}
can be sampled resulting in an algorithm that is similar to GTD($\lambda$), but differs in its update to the primary weights:
\begin{equation}\label{eq:GTD2}
\vecw_{t+1} \leftarrow ~\vecw_t + \alpha (\vech_t^{\tr}\vecx_t)\vecx_t - \alpha \gamma_{t+1} (1-\lambda)(\vech_t^{\tr}\vecz^\rho_t)\vecx_{t+1}
.
\end{equation}
%
This update does not make use of the TD-error $\delta_t$, except through the secondary weights $\vech$. The GTD2($\lambda$) algorithm performs stochastic gradient descent on the linear $\mspbe$, unlike GTD($\lambda$), which uses an approximate gradient, as we discuss further in Section \ref{sec_saddlepoint} when describing the Saddlepoint methods.



\subsection[Hybrid]{Hybrid TD methods}
The Hybrid TD methods were created to achieve the data efficiency of TD($\lambda$) when data is sampled on-policy, and the stability of Gradient-TD methods when the data is sampled off-policy. Early empirical experience with TD(0) and GTD(0) in on-policy problems suggested that TD(0) might be more sample efficient \citep{sutton2009fast}. Later studies highlighted the need for additional empirical comparisons to fully characterize the relative strengths of GTD($\lambda$) compared with TD($\lambda$) \citep{dann2014policy, white2016investigating}.
% MARTHA: Why remove this? I sort of liked it
%Nevertheless, we do know the choice of stepsize parameter values for GTD($\lambda$) is strongly problem dependent: in some off-policy problems like Baird's counter example $\alpha_h$ must be larger than $\alpha$ to achieve good performance, and in other problems the reverse is true (White \& White, 2016). This suggests that a method that could perform TD-updates when the data is on-policy, might exhibit less sensitivity in it's performance to the choice of $\alpha_h$---perhaps $\alpha_h > \alpha$ would always be best.

Hybrid TD methods were first proposed by \citet{maei2011gradient} and \citet{hackman2013faster} and were further developed to make use of eligibility traces by \citet{white2016investigating}. The derivation of the method starts with the gradient of the excursion linear $\mspbe$.
Recall from Equation \eqref{eq:MSPBE} that the linear $\mspbe$ can be written $(\vecb \sneg\Amat \vecw)^\top \Cmat^\inv (\vecb \sneg\Amat \vecw)$. The matrix $\Cmat$ is simply the weighting in the squared error for $\vecb \sneg\Amat \vecw$. In fact, because we know every solution to the linear $\mspbe$ satisfies $\vecb \sneg\Amat \vecw = \zerovec$, the choice of $\Cmat$ asymptotically is not relevant, as long as it is positive definite. The gradient of the linear $\mspbe$, $\sneg\Amat^\top  \Cmat^\inv (\vecb \sneg\Amat \vecw)$ can therefore be modified to $\sneg\Amat^\top  \Bmat (\vecb \sneg\Amat \vecw)$, for any positive definite $\Bmat$, and should still converge to the same solution(s).


In order to achieve a hybrid learning rule, this substitution must result in an update that reduces to the TD($\lambda$) update when $\pi = b$.
This can be achieved by setting $\Bmat = \mathbb{E}_{d_b} \biggl[ \bigl(\vecx_t - \gamma_{t+1} \vecx_{t+1}\bigr)\vecz_t\biggr]$, which is the $\Amat$ matrix for the behavior. Because this $\Bmat$ is estimated with on-policy samples---since we are following $b$---we know $\Bmat$ is positive semi-definite \citep{sutton1988learning}, and positive definite under certain assumptions on the features. Further, when $b = \pi$, we have that   $\Bmat = \Amat^{-\top}$, giving update
$\sneg\Amat^\top  \Bmat (\vecb \sneg\Amat \vecw) = \vecb \sneg\Amat \vecw$. The TD($\lambda$) update is a stochastic sample of expected update $\vecb \sneg\Amat \vecw$, and so when HTD($\lambda$) uses a stochastic sample of $\sneg\Amat^\top  \Bmat (\vecb \sneg\Amat \vecw)$ when $b = \pi$, it is in fact using the same update as TD($\lambda$).

The HTD($\lambda$) algorithm is:
\begin{align}\label{eq:HTD}
\vech_{t+1} \leftarrow& ~\vech_t + \alpha_h\biggl[\delta_t\vecz^\rho_t - (\vecx_t - \gamma_{t+1}\vecx_{t+1})(\vech_t^{\tr}\vecz_t)  \biggr] \nonumber\\\
\vecw_{t+1} \leftarrow& ~\vecw_t + \alpha\biggl[\delta_t\vecz^\rho_t - (\vecx_t - \gamma_{t+1}\vecx_{t+1})(\vecz^\rho_t -\vecz_t)^{\tr}\vech_t  \biggr]
\end{align}
HTD($\lambda$) has two eligibility trace vectors, with $\vecz$ being a conventional accumulating eligibility trace for the behavior policy. If $\pi=b$, then all the $\rho_t$ are 1 and $\vecz_t = \vecz^\rho_t$, which causes the last term in the $\vecw$ update to be zero and the overall update reduces to the TD($\lambda$) algorithm. The last term in the $\vecw$ update applies a correction to the usual Off-policy TD($\lambda$).

Like GTD($\lambda$), the HTD($\lambda$) algorithm is a posterior correction method that should converge to the minimum of the excursion variant of the linear $\mspbe$. No formal stochastic approximation results have been published, though the expected update is clearly convergent because $\Amat^\top \Bmat \Amat$ is positive semi-definite. This omission is likely due to the mixed empirical results achieved with Hybrid TD methods Markov chains and random MDPs \citep{hackman2013faster,white2016investigating}.


\subsection{Gradient-TD methods based on a saddlepoint formulation}\label{sec_saddlepoint}

Optimization of the linear $\mspbe$ can be reformulated as a saddle point problem, yielding another family of stable Off-policy TD methods based on gradient descent.
%Several Gradient-TD algorithms have been developed based on reformulating the linear $\mspbe$ as a saddlepoint problem.
These include the original Proximal-GTD methods \citep{liu2016proximal, liu2020finitesample} methods, stochastic variance reduction methods for policy evaluation \citep{du2017stochastic}, and gradient formulations of Retrace and Tree Backup \citep{touati2018convergent}.
The linear $\mspbe$ can be rewritten using convex conjugates:
%
\begin{equation}\label{eq:saddleMSPBE}
\text{linear $\mspbe$}(\vecw) = \min_{\vech} (\vecb -\Amat \vecw)^\top \vech - \tfrac{1}{2} \| \vech \|_\Cmat^2
\end{equation}
%
where the weighted norm $\| \vech \|_\Cmat^2 = \vech^\top \Cmat \vech$.

% were proposed to improve on Gradient-TD methods theoretically. Although Gradient-TD methods (Sutton et al.,\ 2009) are derived from the gradient of an objective function, they are not true stochastic gradient descent methods with respect to their objective function (Szepesvari, 2011).



The utility of this saddlepoint formulation is that it removes the product of expectations, with the explicit addition of an auxiliary variable.
This avoids the double sampling problem, since for a given $\vech$, it is straightforward to sample $(\vecb -\Amat \vecw)^\top \vech$ (see Equation \eqref{eq_td_A}) with sample $\delta_t {\vecz_t^{\rho}}^\top \vech$. It is similarly straightforward to sample the gradient of this objective for a given $\vech$.
Now this instead requires that this auxiliary variable $\vech$ be learned. The resulting algorithm is identical to GTD2(0) when using stochastic gradient descent for this saddle point problem. This result is somewhat surprising, because GTD2(0) was derived from the gradient of the linear $\mspbe$ using a quasi-stationary estimate of a proportion of the gradient.

The saddle point formulation---because it is a clear convex-concave optimization problem---allows for many algorithmic variants. For example, stochastic gradient descent algorithm for this convex-concave problem can incorporate accelerations, such as mirror-prox---as used by \citet{liu2020finitesample} variance reduction approaches---as used \citep{du2017stochastic}. This contrasts the original derivation for GTD2($\lambda$), which used a quasi-stationary estimate and was not obviously a standard gradient descent technique. One such accelerated algorithm is Proximal GTD2($\lambda$), described by the following update equations:
\begin{align}\label{Proximal GTD2}
%\delta_t ~\defeq~& R_{t+1} + \gamma_{t+1}\vecw_t^{\tr}\vecx_{t+1} - \vecw_t^{\tr}\vecx_{t}\nonumber\\
%\vecz^\rho_t \leftarrow& ~\rho_t(\gamma_t \lambda_t \vecz^\rho_{t-1}  +\vecx_t)\nonumber\\
\vech_{t+\frac{1}{2}} \leftarrow& ~\vech_{t} + \alpha_\vech \biggl[\delta_{t} \vecz_t^{\rho} - (\vech_{t}^{\tr}\vecx_t)\vecx_t\biggr]\\
\vecw_{t+\frac{1}{2}} \leftarrow& ~\vecw_t +\alpha (\vech_t^{\tr}\vecx_t)\vecx_t -\alpha \gamma_{t+1} (1 - \lambda_{t+1}) (\vech_t^{\tr}\vecz_{t}^{\rho} ) \vecx_{t+1}\\
\delta_{t+\frac{1}{2}} ~\defeq~& R_{t+1} + \gamma_{t+1} \vecw_{t+\frac{1}{2}}^{\tr}\vecx_{t+1} - \vecw_{t+\frac{1}{2}}^{\tr}\vecx_{t}\\
\vech_{t+1} \leftarrow& ~\vech_{t} + \alpha_\vech \biggl[\delta_{t+\frac{1}{2}} \vecz_t^\rho - (\vech_{t+\frac{1}{2}}^{\tr}\vecx_t)\vecx_t\biggr]\\
\vecw_{t+1} \leftarrow& ~\vecw_t +\alpha (\vech_{t+\frac{1}{2}}^{\tr}\vecx_t)\vecx_t -\alpha  \gamma_{t+1} (1 - \lambda_{t+1}) (\vech_{t+\frac{1}{2}}^{\tr}\vecz_{t}^{\rho} ) \vecx_{t+1}
\end{align}
%
%The unfamiliar double-update to the $\vecw$ and $\vech$, denoted by subscripts ${t+\frac{1}{2}}$ and $t+1$, correspond to one of the gradient accelerations mentioned above.
The double update to $\vecw$ and $\vech$, denoted by subscripts ${t+\frac{1}{2}}$ and $t+1$, is produced by applying the Stochastic Mirror-Prox acceleration \citep{juditsky2011solving} to the gradient descent update derived from Equation \ref{eq:saddleMSPBE}. We will refer to this algorithm by the shorthand name PGTD2 in the figures.


The saddle point formulation cannot be applied to derive an accelerated version of GTD($\lambda$). %This contrasts the GTD methods, which use a quasi-stationary estimates and so are not true stochastic gradient descent methods.
Recall that GTD($\lambda$) was obtained by reordering expectations in the gradient of the linear $\mspbe$, and then using quasi-stationary estimates of different expected values. This alternative formulation cannot obviously be written as a saddle point problem---though it has nonetheless been shown to be convergent. %In this way, the saddlepoint and quasi-stationary approaches have complementary roles to play.
Nevertheless, a heuristic approximation of accelerated Proximal GTD($\lambda$) has been proposed \citep{liu2020finitesample}, and its update equations are similar to that of Proximal GTD2($\lambda$) with difference in updating the weight vector $\vecw$:
\begin{align}\label{Proximal GTD}
\vecw_{t+\frac{1}{2}} \leftarrow& ~\vecw_t +\alpha \delta_{t} \vecz_t^{\rho} -\alpha \gamma_{t+1} (1 - \lambda_{t+1}) (\vech_{t}^{\tr}\vecz_{t}^{\rho} ) \vecx_{t+1} \\
\vecw_{t+1} \leftarrow& ~\vecw_t +\alpha \delta_{t+\frac{1}{2}} \vecz_t^\rho - \alpha \gamma_{t+1} (1 - \lambda_{t+1}) (\vech_{t+\frac{1}{2}}^{\tr}\vecz_t^\rho) \vecx_{t+1}
\end{align}
We will refer to this algorithm by the shorthand name PGTD in the figures.

Both Proximal GTD($\lambda$) and Proximal GTD2($\lambda$) minimize the excursion variant of linear $\mspbe$, as they assume $d = d_b$.
%Inspecting the trace updates in (\ref{Proximal GTD2}) we can see that both Proximal methods use only posterior corrections.
% \adam{I propose we omit the following sentence because we could also make alt like TDC but we do't talk about that.}
% MARTHAC: I think it matches because we have the table now
The idea of the saddlepoint formulation, however, is more general and alternatives weightings could be considered, such as $d = d_\pi$ (shown in Table 1). The expectations in the linear $\mspbe$ would simply change, and prior corrections would need to be incorporated
% into the estimate of $\Amat$ and $\vecb$ or into $\delta_t \vecx_t$
to get an unbiased sample of $\vecb -\Amat\vecw$ weighted by $d_\pi$.

The practical utility of these methods for online estimation is still not well understood. Several of the accelerations mentioned above, such as the use of stochastic variance reduction strategies \citep{du2017stochastic}, assume a batch learning setting. The online algorithms, as mentioned, all use variants of GTD2($\lambda$), which seems to perform more poorly than GTD($\lambda$) in practice \citep{touati2018convergent}. This saddle point formulation, however, does enable continued advances in online convex optimization to be ported to reinforcement learning. Additionally, this formulation allows analysis tools from optimization to be applied to the analysis of TD learning methods. For example,  \citet{touati2018convergent} provided the first finite sample analysis for GTD2($\lambda$), which is not possible with the original GTD2($\lambda$) derivation based on the quasi-stationary secondary weights. %It seem highly likely that more advances in online variance reduction strategies will improve the practical utility of these methods in the future.

\subsection{Off-policy learning with action-dependent boostrapping}
\label{subsct:ABTDDerivation}

A common concern with using importance sampling ratios is the possibility for high variance, due to large ratios.\footnote{We would like to note that, to the best of our knowledge, variance issues due to importance sampling ratios have not been concretely demonstrated in the literature. This concern, therefore, is based on intuition and should be considered a hypothesis rather than a known phenomenon.}
Several methods have been introduced that control this variance, either by explicitly or implicitly avoiding the product of importance sampling ratios in the traces. The Tree Backup($\lambda$) algorithm, which we call TB($\lambda$), was the first off-policy method that did not explicitly use importance sampling ratios \citep{precup2000eligibility}. This method decays traces more, incurring more bias; newer algorithms such as V-trace($\lambda$) and ABQ($\zeta$) attempt to reduce variance but without decaying traces as much, and improve performance in practice. In this section, we describe the state-value prediction variants of TB($\lambda$), V-trace($\lambda$), and ABQ($\zeta$) that we investigate in our empirical study.


These three methods can all be seen as Off-policy TD($\lambda$) with $\lambda$ generalized from a constant to a function of state and action.
This unification was highlighted by \citet{mahmood2017multistep} when they introduced ABQ. This unification makes explanation of the algorithms straightforward: each method simply uses a different action-dependent trace function $\lambda: \States \times \Actions \rightarrow [0,1]$. All three methods were introduced for learning action-values; we present the natural state-value variants below.


We begin by providing the generic Off-policy TD algorithm with action-dependent traces.
The key idea is to set $\lambda_t \defeq \lambda(S_{t-1}, A_{t-1})$ such that $\rho_{t-1} \lambda_t$ is well-behaved. The Off-policy TD($\lambda$) algorithm for this generalized trace function can be written\footnote{This update explicitly uses $\rho_t$ in the update to $\vecw_{t+1}$. This contrasts the earlier Off-policy TD updates in Equation \eqref{eq:offTD}, which have $\rho_t$ in the trace. These two forms are actually equivalent, in that the update to $\vecw$ is exactly the same. We show this equivalence in Appendix~\ref{app_importancesampling}. We use this other form here, to more clearly highlight the relationship between $\rho_{t-1}$ and $\lambda_t$.}
%
\begin{align}
\vecw_{t+1} & = \vecw_t +\alpha \rho_t \delta_t \vecz_t \nonumber \\
\vecz_t & = \gamma_t \rho_{t-1} \lambda_t \vecz_{t-1} + \vecx_{t}\label{eq:OffTDTrace}
,
\end{align}
%
Now we can specify different algorithms using this generic variant of Off-policy TD($\lambda$), by specifying different implementations of the $\lambda$ function.
Like Off-policy TD($\lambda$), these algorithms all perform only posterior corrections.

TB($\lambda$) is Off-policy TD($\lambda$) with $\lambda_t = b_{t-1} \lambda$, for some tuneable constant $\lambda \in [0,1]$. Replacing $\lambda_t$ with $b_{t-1} \lambda$ in the eligibility trace update in Equation \ref{eq:OffTDTrace} simplifies as follows:
%
\begin{align}
\vecz_t & = \gamma_t \frac{\pi_{t-1}}{b_{t-1}} b_{t-1}\lambda \vecz_{t-1} + \vecx_{t} \nonumber \label{eq:TBTrace}\\
&=\gamma_t \pi_{t-1}\lambda\vecz_{t-1}+\vecx_{t},
\end{align}
%
and gives the state-value variant of TB($\lambda$).

A simplified variant of the V-trace($\lambda$) algorithm \citep{espeholt2018impala} can be derived with a similar substitution: $\lambda_t = \min\left(\frac{\bar{c}}{\pi_{t-1}},\frac{1}{b_{t-1}}\right) \lambda b_{t-1}$, where $\bar{c} \in \mathbb{R}^+$ and $\lambda \in [0,1]$ are both tuneable constants. The eligibility trace update becomes:
%
\begin{align}
\vecz_t & = \gamma_t \min \left(\frac{\bar{c}}{\pi_{t-1}},\frac{1}{b_{t-1}}\right) \lambda b_{t-1} \frac{\pi_{t-1}}{b_{t-1}} \vecz_{t-1} + \vecx_{t} \nonumber\\
&= \gamma_t \min \left(\frac{\bar{c}}{\pi_{t-1}},\frac{1}{b_{t-1}}\right) \lambda \pi_{t-1} \vecz_{t-1} + \vecx_{t} \nonumber\\
&= \gamma_t \min \left(\frac{\bar{c}\pi_{t-1}}{\pi_{t-1}},\frac{\pi_{t-1}}{b_{t-1}}\right) \lambda \vecz_{t-1} + \vecx_{t} \nonumber\\
&= \gamma_t \min \left(\bar{c},\rho_{t-1}\right) \lambda \vecz_{t-1} + \vecx_{t}
\label{eq:V-traceTrace}
,
\end{align}
%
The parameter $\bar{c}$ is used to cap importance sampling ratios in the trace.
Note that it is not possible to recover the full V-trace($\lambda$) algorithm in this way. The more general V-trace($\lambda$) algorithm uses an additional parameter, $\bar{\rho} \in \mathbb{R}^+$ that caps the $\rho_t$ in the update to $\vecw_{t+1}$: $\min(\bar{\rho},\rho_t) \delta_t \vecz_t$. When $\bar{\rho}$ is set to the largest possible importance sampling ratio, it does not affect $\rho_t$ in the update to $\vecw_t$ and so we obtain the equivalence above. For smaller $\bar{\rho}$, however, V-trace($\lambda$) is no longer simply an instance of Off-policy TD($\lambda$). In the experiments that follow, we investigate this simplified variant of V-trace($\lambda$) that does not cap $\rho_t$ and set $\bar{c}=1$ as done in the original Retrace algorithm.


ABTD($\zeta$) for $\zeta \in [0,1]$ uses $\lambda_t = \nu_{t-1}b_{t-1}$, with the following eligibility trace update:
%
\begin{align}
\vecz_t & = \gamma_t \frac{\nu_{t-1}}{b_{t-1}} b_{t-1}\lambda \vecz_{t-1} + \vecx_{t} \nonumber \label{eq:ABTDTrace}\\
&=\gamma_t \nu_{t-1}\pi_{t-1}\vecz_{t-1}+\vecx_{t}.
\end{align}
%
with the following scalar parameters to define $\nu_t$
%
\begin{align*}
\nu_t &\defeq \nu(\psi(\zeta), s_t, a_t) \defeq \min \left(\psi(\zeta),\frac{1}{\max(b(a_t|s_t),\pi(a_t|s_t))}\right)\\
\psi(\zeta) &\defeq 2\zeta\psi_0 + \max(0,2\zeta - 1) (\psi_{\text{max}} - 2\psi_0)\\
\psi_{0} &\defeq \frac{1}{\max_{s, a}\max(b(a|s),\pi(a|s))}\\
\psi_{\textnormal{max}} &\defeq \frac{1}{\min_{s, a}\max(b(a|s),\pi(a|s))}
.
\end{align*}

The convergence properties of all three methods are similar to  Off-policy TD($\lambda$). They are not guaranteed to converge under off-policy sampling with weighting $d_b$ and function approximation. With the addition of gradient corrections similar to GTD($\lambda$), these algorithms are convergent. For explicit theoretical results, see Mahmood et al. (2017) for ABQ with gradient correction and Touati et al. (2018) for convergent versions of Retrace and Tree Backup.


\subsection[ETD and ETDBeta]{Emphatic-TD learning}
\label{sec:etd}

Emphatic Temporal Difference learning, ETD($\lambda$), provides an alternative strategy for obtaining stability under off-policy sampling without computing gradients of the linear $\mspbe$.  The key idea is to incorporate some prior corrections so that the weighting $d$ results in a positive definite matrix $\Amat$. Given such an $\Amat$, a TD($\lambda$) algorithm---a semi-gradient algorithm---can be shown to converge. Importantly, this allows for a stable off-policy algorithm with only a single set of weights. Gradient-TD methods, on the other hand, use two stepsize parameters and two weight vectors to achieve stability.
%
In this section, we describe two different variants of Emphatic-TD methods: ETD($\lambda$) and ETD($\lambda,\,\beta$), which was introduced to reduce the variance of ETD($\lambda$).

ETD($\lambda$) minimizes a variant of the linear $\mspbe$ defined in Equation \ref{eq:MSPBE}, where the weighting $d$ is defined based on the {\em followon} weighting. The followon reflects (discounted) state visitation under the target policy when doing excursions from the behavior: starting from states sampled according to $d_b$. The followon is defined as
\begin{equation}
f(s_t)\defeq d_b(s_t) + \gamma(s_t) \sum_{s_{t-1}, a_{t-1}}d_b(s_{t-1})\pi(a_{t-1}|s_{t-1})P(s_t | s_{t-1}, a_{t-1}) + \hdots \label{eq:ETDF}
.
\end{equation}
The emphatic weighting then corresponds to $m(s_t) = d_b(s_t) \lambda + (1-\lambda) f(s_t)$. This is the weighting used in the linear $\mspbe$ in Equation \ref{eq:MSPBE}, setting $d(s) = m(s)$.

The Emphatic TD($\lambda$) algorithm is specified by the following equations:
\begin{align*}
%\delta_t ~\defeq~& R_{t+1} + \gamma_{t+1}\vecw_t^{\tr}\vecx_{t+1} - \vecw_t^{\tr}\vecx_{t}\nonumber\\
F_t \leftarrow& ~\rho_{t-1}\gamma_t F_{t-1} + 1\\
M_{t}  \leftarrow& \lambda_t + (1 - \lambda_t)F_t\\
\vecz_t^{\rho} \leftarrow& ~\rho_t \left(\gamma_t \lambda \vecz_{t-1}^{\rho} + M_t \vecx_{t}\right)\\
\vecw_{t+1} \leftarrow& ~ \vecw_t +\alpha \delta_t \vecz_t^{\rho}
,
\end{align*}
\noindent with $F_0=1$ and $\vecz_0^{\rho}=\vec0$. The scalar estimate $F_t$ is used to include the weighting defined in Equation \ref{eq:ETDF}.
 %and $I_t$ is shorthand for the interest in state $S_t$ . We can write the update for $F_t$ non-recursively:
 %
 To gain some intuition for this weighting, consider a setting where $\gamma_t =\gamma$ is constant and $\lambda = 0$. Then $M_t = F_t =  \sum_{j=0}^{t}{\gamma^j\prod_{i=1}^{j}\rho_{t-i}} $, giving trace $\vecz_t^{\rho} \leftarrow ~\rho_t \left(\gamma_t \lambda \vecz_{t-1}^{\rho} + \sum_{j=0}^{t}{\gamma^j\prod_{i=1}^{j}\rho_{t-i}} \vecx_{t}\right)$.

There are some similarities to the weighting in the Alternative-life TD($\lambda$) trace in Equation \ref{eq:precup2001}, where $\vecz_t^{\rho} \leftarrow ~\rho_t \left(\gamma_t \lambda \vecz_{t-1}^{\rho} + \prod_{i=1}^{t}\rho_{i} \vecx_{t}\right)$. Both adjust the weighting on $\vecx_t$ to correct for---or adjust---the state distributions. Alternative-Life TD more aggressively downweights states that would not have been visited under the target policy. ETD, on the other hand, reweights based on how frequently the states would be seen when starting $\pi$ as an excursion from $b$.

Emphatic TD($\lambda$) has strong convergence guarantees in the case of linear function approximation. The ETD($\lambda$) under off-policy training has been shown to converge in expectation using the same expected update analysis used to show that TD($\lambda$) converges under on-policy training. Later, \citet{yu2015convergence} extended this result to show that ETD($\lambda$) converges with probability one. Perhaps more practically relevant, this weighting also resolves the issues raised by Kolter's example (2011). Kolter's example demonstrated that for a particular choice of $\pi$ and $b$, the solution to the linear $\mspbe$ could result in arbitrarily bad error compared with the best possible approximation in the function class. In other words, even if the true value function can be well approximated by the function class, the off-policy fixed point from the linear $\mspbe$ with weighting $d = d_b$ can result in an arbitrarily poor approximation to the values. \citet{hallak2016generalized} showed that the fixed points of the linear $\mspbe$ with the emphatic weighting, on the other hand, do not suffer from this problem (see their Corollary 1). This result was actually generally shown for an extended ETD($\lambda$) method, called ETD($\lambda, \beta$), which we describe next.

ETD($\lambda$) was extended to include an additional scalar tuneable parameter $\beta$, to further control variance due to prior corrections. The ETD($\lambda,\,\beta$) algorithm updates are identical to ETD($\lambda$) except for the update to $F_t$:
\begin{equation*}
F_t \leftarrow ~\rho_{t-1}\beta F_{t-1} + 1
\end{equation*}
%
If $\beta = \gamma$, then the update is identical to ETD($\lambda$). If $\beta = 0$, then the update is identical to Off-policy TD($\lambda$), and there are a spectrum of methods in between. This $\beta$, then, introduces bias to reduce variance in the followon trace for ETD. \citet{hallak2016generalized} showed that $\beta$ can be less than $\gamma$, and ETD($\lambda,\beta$) can still enjoy the convergence properties of ETD($\lambda$), depending on the mismatch between the target and behavior policy. For more similar policies, $\beta$ can be closer to zero and still converge: it can behave like Off-policy TD($\lambda$) and still converge if the setting is almost on-policy. For a greater mismatch, $\beta$ must be nearer to $\gamma$.
